# Supplementary material for: Hand-4DGS: Feed-Forward 3D Gaussian Splatting for 4D Hand Reconstruction from Egocentric Videos
Source: arXiv:2606.19156 source file (2026-10-07)
Supplement: Supplementary file 1 [file X_suppl.tex]

\ifx\supp\undefined
    \documentclass[runningheads]{llncs}
    
    \usepackage[review,year=2026,ID=13420]{eccv}
    \usepackage{eccvabbrv}
    \usepackage{graphicx}
    \usepackage{booktabs}
    \usepackage[accsupp]{axessibility}  % Improves PDF readability for those with 
    
    % Import additional packages in the preamble file, before hyperref
    % \input{preamble}
    
    % It is strongly recommended to use hyperref, especially for the review version.
    % hyperref with option pagebackref eases the reviewers' job.
    % Please disable hyperref *only* if you encounter grave issues, 
    % e.g. with the file validation for the camera-ready version.
    %
    % If you comment hyperref and then uncomment it, you should delete *.aux before re-running LaTeX.
    % (Or just hit 'q' on the first LaTeX run, let it finish, and you should be clear).
    % \definecolor{cvprblue}{rgb}{0.21,0.49,0.74}
    % \usepackage[pagebackref,breaklinks,colorlinks,allcolors=cvprblue]{hyperref}
    
    \usepackage{kotex}          % for quick comment in Korean
    \usepackage{duckuments}
    \usepackage{multirow} 
    \usepackage{ulem}
    \input{macro}
    
    %%%%%%%%% TITLE - PLEASE UPDATE
    \title{Feed-Forward 3D Gaussian Splatting
    for 4D \\ Hand Reconstruction from Egocentric Videos}

    %%%%%%%%% AUTHORS - PLEASE UPDATE

    \author{First Author\inst{1}\orcidlink{0000-1111-2222-3333} \and
    Second Author\inst{2,3}\orcidlink{1111-2222-3333-4444} \and
    Third Author\inst{3}\orcidlink{2222--3333-4444-5555}}
    
    % TODO FINAL: Replace with an abbreviated list of authors.
    % \authorrunning{F.~Author et al.}
    % First names are abbreviated in the running head.
    % If there are more than two authors, 'et al.' is used.
    
    % TODO FINAL: Replace with your institution list.
    \institute{Princeton University, Princeton NJ 08544, USA \and
    Springer Heidelberg, Tiergartenstr.~17, 69121 Heidelberg, Germany
    \email{lncs@springer.com}\\
    \url{http://www.springer.com/gp/computer-science/lncs} \and
    ABC Institute, Rupert-Karls-University Heidelberg, Heidelberg, Germany\\
    \email{\{abc,lncs\}@uni-heidelberg.de}}

    \begin{document}
    
    % supplementary settings
    \makeatletter
    \renewcommand{\maketitle}{%
        \author{Supplementary Material}%
        \titlerunning{ECCV 2026 Submission \#13420}%
        \authorrunning{ECCV 2026 Submission \#13420}%
        \institute{}%
        \maketitleold%
    }
    \makeatother
    \maketitle%supplementary

\else
    \clearpage
    \setcounter{page}{1}
    \let\twocolumn\oldtwocolumn  % 
    % \maketitlesupplementary
\fi

\renewcommand{\thesection}{\Alph{section}}
\setcounter{section}{0}
\renewcommand{\thetable}{S\arabic{table}}
\renewcommand{\thefigure}{S\arabic{figure}}
\setcounter{figure}{0}
\setcounter{table}{0}

In the Appendix, we present in-the-wild video results (\sref{sec:in-the-wild}). To further show the robustness and applicability of our framework, we provide results using detector-based bounding boxes and alternative hand pose estimator (\sref{sec:robust}). In \sref{sec:details_supp}, we describe further implementation details and training setups. Finally, \sref{sec:supp_qual} provides extended qualitative results on H2O and ARCTIC datasets.

%%%%%%%%%%%%%%%%%%%%%%%%%%%%%%%%%%%%%%
%%%%%%%%%%%%%%%%%%%%%%%%%%%%%%%%%%%%%%

\section{In-The-Wild Results}
\label{sec:in-the-wild}

To demonstrate the generalizability of \ours, \fref{fig:supp_in-the-wild} presents inference results for various in-the-wild clips from the HoloAssist\cite{wang2023holoassist} dataset. Even on unseen poses and backgrounds, the model yields plausible hand reconstructions through direct feed‑forward inference. For each sequence, we apply 100 TTO steps to reduce color shift, which takes only a few seconds.
\input{figs/fig_supp_in-the-wild}
%%%%%%%%%%%%%%%%%%%%%%%%%%%%%%%%%%%%%%
%%%%%%%%%%%%%%%%%%%%%%%%%%%%%%%%%%%%%%

\section{Robustness Analysis of Hand‑4DGS}
\label{sec:robust}

In this section, we evaluate the robustness of Hand‑4DGS under variations in training settings. \tref{tab:supp_pose} examines the effect of different pose estimators, showing that our framework consistently improves over both HaMeR~\cite{pavlakos2024reconstructing} and WiLoR~\cite{potamias2025wilor} and maintains stable reconstruction quality across estimators. \tref{tab:supp_bbox} examines training with detector‑based bounding boxes (denoted as w\slash o GT bbox), which are less accurate and include non-negligible failure cases. Even under this noisier setting, Hand‑4DGS preserves stable reconstruction quality with limited performance degradation, demonstrating robustness to variations in bounding‑box quality.

\input{supp_assets/tables/supp_pose}
\input{supp_assets/tables/supp_bbox}

%%%%%%%%%%%%%%%%%%%%%%%%%%%%%%%%%%%%%%
%%%%%%%%%%%%%%%%%%%%%%%%%%%%%%%%%%%%%%

\section{Experimental Details}
\label{sec:details_supp}

\subsection{Data Processing and Feature Extraction}
\label{supp:exp:data}

For feature extraction, we use pretrained ViT from HaMeR. We resize the input image cropped with the given bounding box to $256 \times 256$ to get $N_t=256$ tokens. For efficiency, we pre-store and load the hand masks, vertices $\mathcal V_{\text{pseudo}}$ from HaMeR, and image backbone token features $z_t \in \mathbb{R}^{N_t \times D_t}$ for training. On average, this process takes about 1 minute for a 500-frame video sequence of resolution $1280 \times 720$ from the H2O dataset.

\subsection{Training Setup and Model Architecture}
\label{supp:exp:arch}

To ensure a fair comparison of 3D hand reconstruction without access to ground truth 3D labels, we use a pre-trained HaMeR model without any fine-tuning on the H2O and ARCTIC datasets in our method and the baselines.
On the H2O dataset, Hand-4DGS is trained at its original resolution of $1280 \times 720$, while on the ARCTIC dataset, Hand-4DGS is trained on downsampled images at a resolution of $1400 \times 1000$. 
We perform training and evaluation only when both hands are sufficiently visible in the image. 
Specifically, we exclude instances where more than half of a bounding box area is outside the image or when HaMeR fails to detect both hands correctly. 
To focus on the evaluation of dynamic region, we compute the PSNR and SSIM between the cropped ground truth images and renderings using the bounding box of each hand, followed by averaging the results.
Additionally, since hands are not visible at the beginning and end of the ARCTIC video sequences, we exclude the first and last 100 frames for each video sequence.

To constrain the wide range of token features $z_t$ from the frozen image backbone model, we empirically adjust the extracted features by applying $\text{sigmoid}(\cdot)-0.5$. We use separate TC layers and MLPs for each hand to predict MANO parameters, translations, and vertex embeddings. 
We set the output channel $D'$ of the TC layer to $16$. To predict global translation from locally cropped image features, we provide the normalized bounding box coordinates as an additional input to $\text{MLP}_\text{trans}(\cdot)$. Following 3DGS, we initialize and optimize the Gaussian scales jointly with Hand-4DGS, and define the final scale as the sum of the optimized scale and the scale $s$ predicted by $\text{MLP}_{\text{scale}}$.
Since the Gaussian scales have a small range, we use the $\texttt{tanh}$ activation function to prevent the residual scale $s_\text{res}$ from diverging. Finally, we initialize the weights and biases of the last layer in MLPs to zero.

\subsection{Training and Inference}
\label{supp:exp:runtime}

For HUGS, training a single scene takes about 15 minutes, whereas EVA requires 24 minutes. Note that for EVA, we remove the existing template alignment process and directly use HaMeR predictions as the initial pose. For a fair comparison, the Hand-4DGS (Per-Video) model is trained for 30K steps on a single scene, with image supervision incorporated after the first 20K steps. The total training time is about 15 minutes. The Hand-4DGS (Generalized) model is trained for 1.3M steps in total, which takes around 41 hours. After training, our generalized model can immediately produce plausible hand reconstructions by directly taking novel scene videos as input, rendering about 1K frames in 18 seconds from H2O videos. Additionally, applying optional test-time optimization with 500 iterations for each test scenes takes less than one minute on a single NVIDIA RTX 4090.

%%%%%%%%%%%%%%%%%%%%%%%%%%%%%%%%%%%%%%
%%%%%%%%%%%%%%%%%%%%%%%%%%%%%%%%%%%%%%

\section{Additional Qualitative Results}
\label{sec:supp_qual}

\fref{fig:supp:h2o} and \fref{fig:supp:arctic} show additional qualitative results on various sequences from the H2O and ARCTIC datasets. Unlike the baselines and Hand-4DGS (Per‑Video), which optimize a separate model for each sequence, Hand-4DGS (Generalized) performs feed‑forward inference on unseen test sequences. Our framework maintains stable geometry across all test cases and achieves superior fidelity in both geometry and appearance compared to baselines.

\fref{fig:main:tc}, \fref{fig:main:vertex}, and \fref{fig:main:generalization} provide qualitative examples for our ablation studies and generalization analysis, which are omitted from the main paper due to space constraints.

\input{figs/fig_anals}
\input{figs/fig_anal_generalization}

\input{figs/fig_supp_hand_pose}
\input{figs/fig_supp_more_h2o}
\input{figs/fig_supp_more_arctic}

\ifx\supp\undefined
    \small
    \clearpage
    \bibliographystyle{splncs04}
    \bibliography{main}
    \end{document}
\fi
